# Supplementary material for: Multimodality Invariant Learning for Multimedia-Based New Item Recommendation
Source: arXiv:2405.15783 source file (2024-04-28)
Supplement: Supplementary file 1 [file appendix.tex]

\section{appendix}
